# Supplementary material for: Multi-Agent Feedback Motion Planning using Probably Approximately Correct Nonlinear Model Predictive Control
Source: arXiv:2501.12234 source file (2025-01-21)
Supplement: Supplementary file 1 [file appendix.tex]

\section{Appendix}

% Tests I could Run to Improve 
% \begin{itemize}
%     \item Run test on the centralized controller
%     \item No Obstacle No Formation Collision Tests (I think I could do up to 10 agents)
%     \item No Formation Collision Tests (Up to 10 Agents)
%     \item Same Obstacle Field Different Starting Positions 
%     \item Different Obstacle Field Different Starting Positions
%     \item Multi-Team Avoidance
% \end{itemize}

Variables
\begin{align}
     \bx_i = ~\begin{bmatrix} x_i y_i \theta_i v_i \phi_i \end{bmatrix}^T\\ x_{obs} = \textbf{a} x_{obs}^i y_{obs}^i
\end{align}

TODO:
\begin{itemize}
    \item Improve Related Work
    \item Get Phoenix Sims up  and  running
    \item Run PACNMPC and MPPI With Flow Field on RRT
    \item 
\end{itemize}
